# Supplementary material for: Collective and nonlinear structure of wind power correlations
Source: arXiv:2602.10136 source file (2026-05-06)
Supplement: Supplementary file 1 [file Supplemental_arXiv.pdf]

# Supplemental Material

## Collective and nonlinear structure of wind power fluctuations

Samy Lakhal,<sup>1,\*</sup> James E. Sardonía,<sup>2</sup> and Mahesh M.Bandi<sup>1,†</sup>

<sup>1</sup>*Nonlinear and Non-equilibrium Physics Unit, OIST Graduate University, Onna 904 0495, Japan*

<sup>2</sup>*Exus Renewables North America, Pittsburgh, Pennsylvania, USA*

### I. DETAILS OF WIND TURBINES

The wind farm analyzed in our study consists of 80 turbines of two different, but similar, models GE2.5-116 and GE2.3-116. The main properties of these turbines are summarized in Tab.I.

TABLE I. Turbine properties provided by the manufacturer.

| Turbine model                  | GE2.5-116 | GE2.3-116 |
|--------------------------------|-----------|-----------|
| Number                         | 73        | 7         |
| Cut-in wind speed [m/s]        | 3         | 3.5       |
| Rated wind speed [m/s]         | 11.5      | 11.0      |
| Reduced power wind speed [m/s] | 26.0      | 22.5      |
| Cut-off wind speed [m/s]       | 31.0      | 31.0      |
| Rated power [MW]               | 2.5       | 2.3       |
| Rotor diameter [m]             | 116       | 116       |
| Rotor height [m]               | 90.0      | 80.0      |

The turbine response curves  $P$  versus  $v$  shown in Fig. 1 exhibit an excellent collapse onto a cubic scaling  $P \propto v^3$ , within cut-in/rated wind-speed values. This good correspondence is the consequence of the 10 min averaging procedure used during sampling, as instantaneous measurements are usually more scattered [1]. Data points deviating from that curve are associated with maintenance periods or exceptional wind conditions.

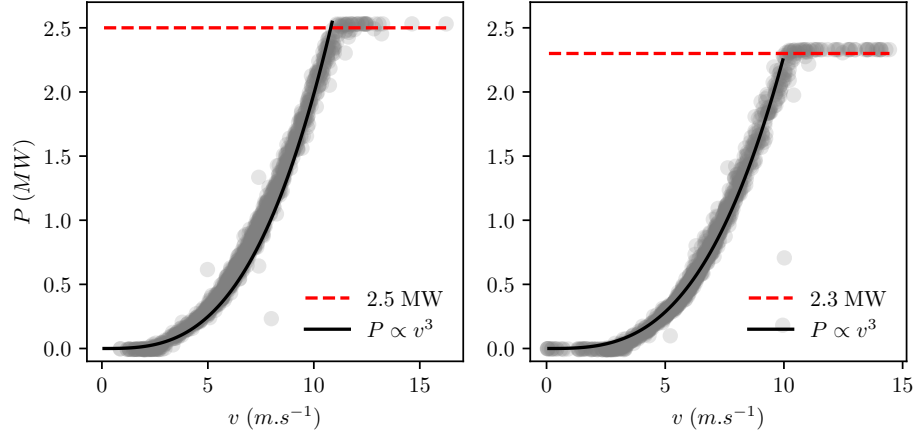

FIG. 1. Power curves  $P$  vs  $v$  sampled for one week for two turbine models, respectively saturating at 2.5 MW for model GE2.5-116 (left) and 2.3 MW for model GE2.3-116(right).

\* samy.lakhal@oist.jp

† bandi@oist.jp

## II. CLEANING OF TURBINE POWER OUTPUT

A substantial fraction of the turbine power output (approximately 40% of the data) lies outside the nominal  $P \propto v^3$  response regime. In practice, the power time series fluctuates within  $0 < P(t) < P_{\text{sat}}$ , constraining increments to  $-P_{\text{sat}} \leq \delta_\tau P \leq P_{\text{sat}}$ . When the wind speed falls outside the operational range, the power saturates at  $P_{\text{sat}}$ , leading to  $\delta_\tau P = 0$ . As a result, the turbine response function affects both the core and the tails of the power-increment statistics, potentially biasing correlation estimates.

To mitigate this effect, we remove power values outside the  $P \propto v^3$  regime, as shown in Fig. 2(a). The resulting cleaned increments, shown in Fig. 2(c), no longer exhibit the excess probability mass at  $(0, \pm P_{\text{sat}})$  visible in Fig. 2(b).

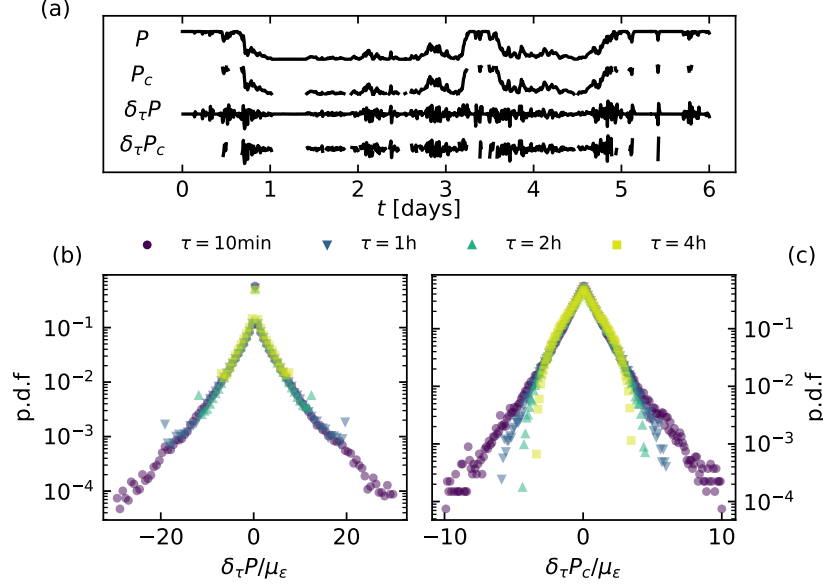

FIG. 2. Wind power  $P$  and cleaned power  $P_c$  statistics. (a) Weekly evolution of  $P$  and  $P_c$ , and their increments ( $\tau = 10$ min). (b), (c) p.d.fs of jumps  $(\delta_\tau P, \delta_\tau P_c)$  for  $\tau = 10$ min, 1h, 2h, 3h. Each plot has been rescaled by a low order ( $\epsilon \ll 1$ ) ratio of empirical and Gaussian moments:  $\mu_\epsilon = \left[ \langle |\delta_\tau X|^\epsilon \rangle \sqrt{\pi} 2^{-\epsilon/2} / \Gamma\left(\frac{1+\epsilon}{2}\right) \right]^{1/\epsilon}$ .

We also compared the statistics of  $v$  and  $P_c^{1/3}$  in Fig. 2. For a given turbine, the two time-series were found to be quasi-identical, both visually in (a), and statistically in (b) and (c). Note, however, that fluctuations beyond rated speed can't be reproduced via filtering.

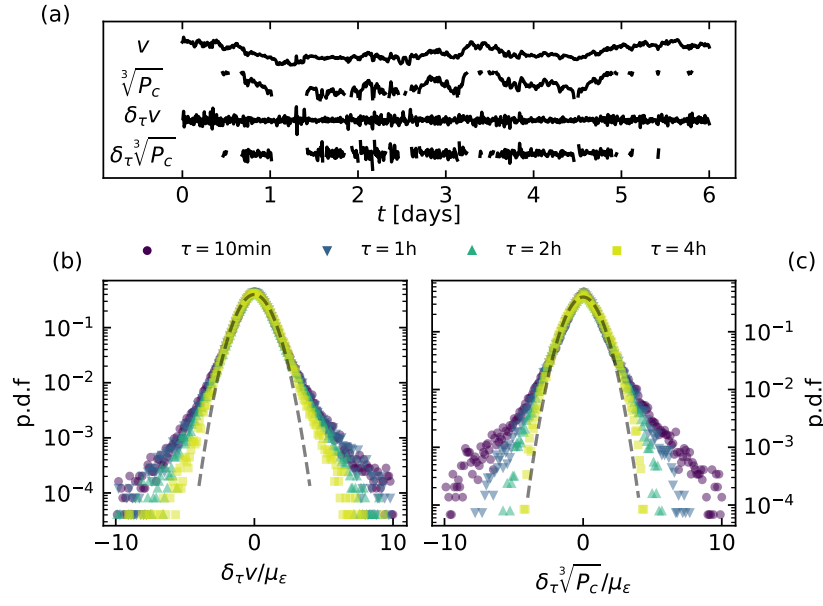

FIG. 3. Same caption as Fig. 2, but for  $(v, \sqrt[3]{P_c})$ . Black curves in (b) and (c) are standardized Gaussian p.d.fs  $\mathcal{N}(0,1)$ .

### III. SCALING OF SINGLE TURBINES

Fig. 4 shows that the second order structure function ( $S_2$ ) of wind speed  $v$  and power  $P$  scale identically among turbines. That behavior generalizes for all orders  $q$ , as is shown in Fig. 5 where scaling exponents  $H_q$  were found to be identical for all turbines.

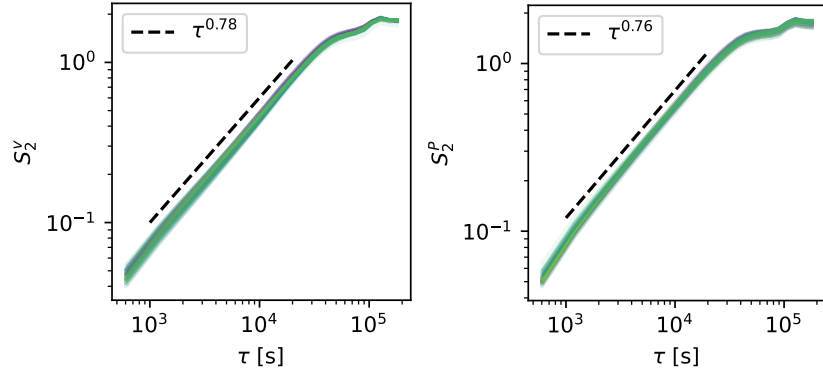

FIG. 4. Structure functions  $S_2(\tau)$  for all 80 turbines of their measured (Left)  $v$  and  $P$  (Right), rescaled vertically to collapse the scaling regime.

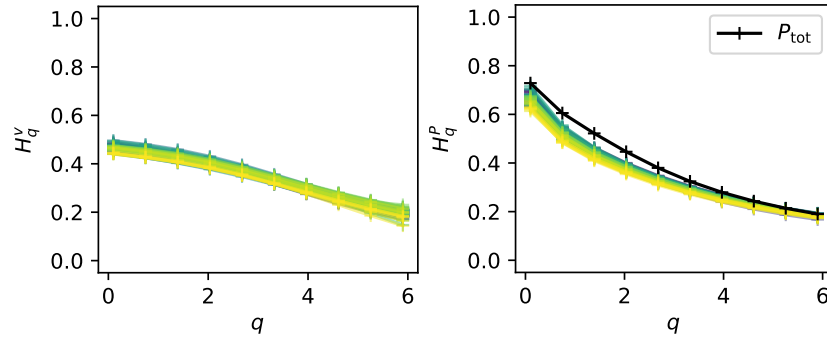

FIG. 5. Generalized exponent spectra  $H_q$ , for all 80 turbines of (Left)  $v$  and (Right)  $P$ ;  $P_{\text{tot}}$  in black.

#### IV. STRUCTURE FUNCTIONS: FROM TURBINE TO FARM OUTPUT

In Fig. 6(main text), we compare the standardized structure functions  $S_q/S_2^{q/2}$  of individual turbines and farm aggregated power output,  $P, P_{\text{tot}}$ . We observe that: (i) curves start collapsing beyond the characteristic sweeping time of the farm  $\tau_S = D/u_{\text{RMS}} = 20\text{km}/5\text{m.s}^{-1} \sim 2\text{h}$  (expectedly from Kraichnan's sweeping hypothesis), and (ii) signals strongly decorrelate around  $T = 24\text{h}$ .

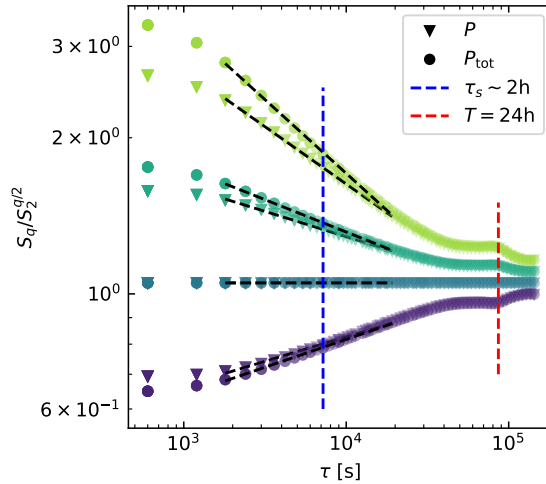

FIG. 6. Rescaled structure functions  $S_q/(S_2)^{q/2}$  for different  $q = 1, 2, 2.5$ , and  $3$  (Bottom to Top). Plots were vertically shifted for visibility.

#### V. BIVARIATE DISTRIBUTIONS OF POWER JUMPS

In the following, we compute the bivariate distribution density of power jumps  $\rho(\delta_\tau P_i, \delta_\tau P_j)$  and show their isolines in Fig. 7 for several lag and turbine distance values  $(\tau, \ell_{ij})$ . We immediately see the strong correlations between neighboring turbines, signed by the diagonal shape of isolines. As  $\tau$  increases, space-time contributions increase cross-correlations, yielding more and more eccentric isolines.

To draw further conclusions on the nonlinearity of correlation structures, we discard the bias of marginal distributions by morphing them into reduced centered Gaussian distributions. Initial distributions being roughly identical for each turbine and fixed  $\tau$ , this morphing operation  $u = \mathcal{F}(\delta P_i)$  is also taken identical. The resulting isolines, shown in Fig. 8, show the presence of correlated extreme events, with progressively decaying sign correlations. Again as  $\tau$  increases, sign correlations increase while extreme events are smoothed out, explaining the diminution of lobes in the  $u_i = -u_j$  direction.

---

[1] M. M. Bandi and J. Apt, Applied Sciences **6** (2016), 10.3390/app6090262.

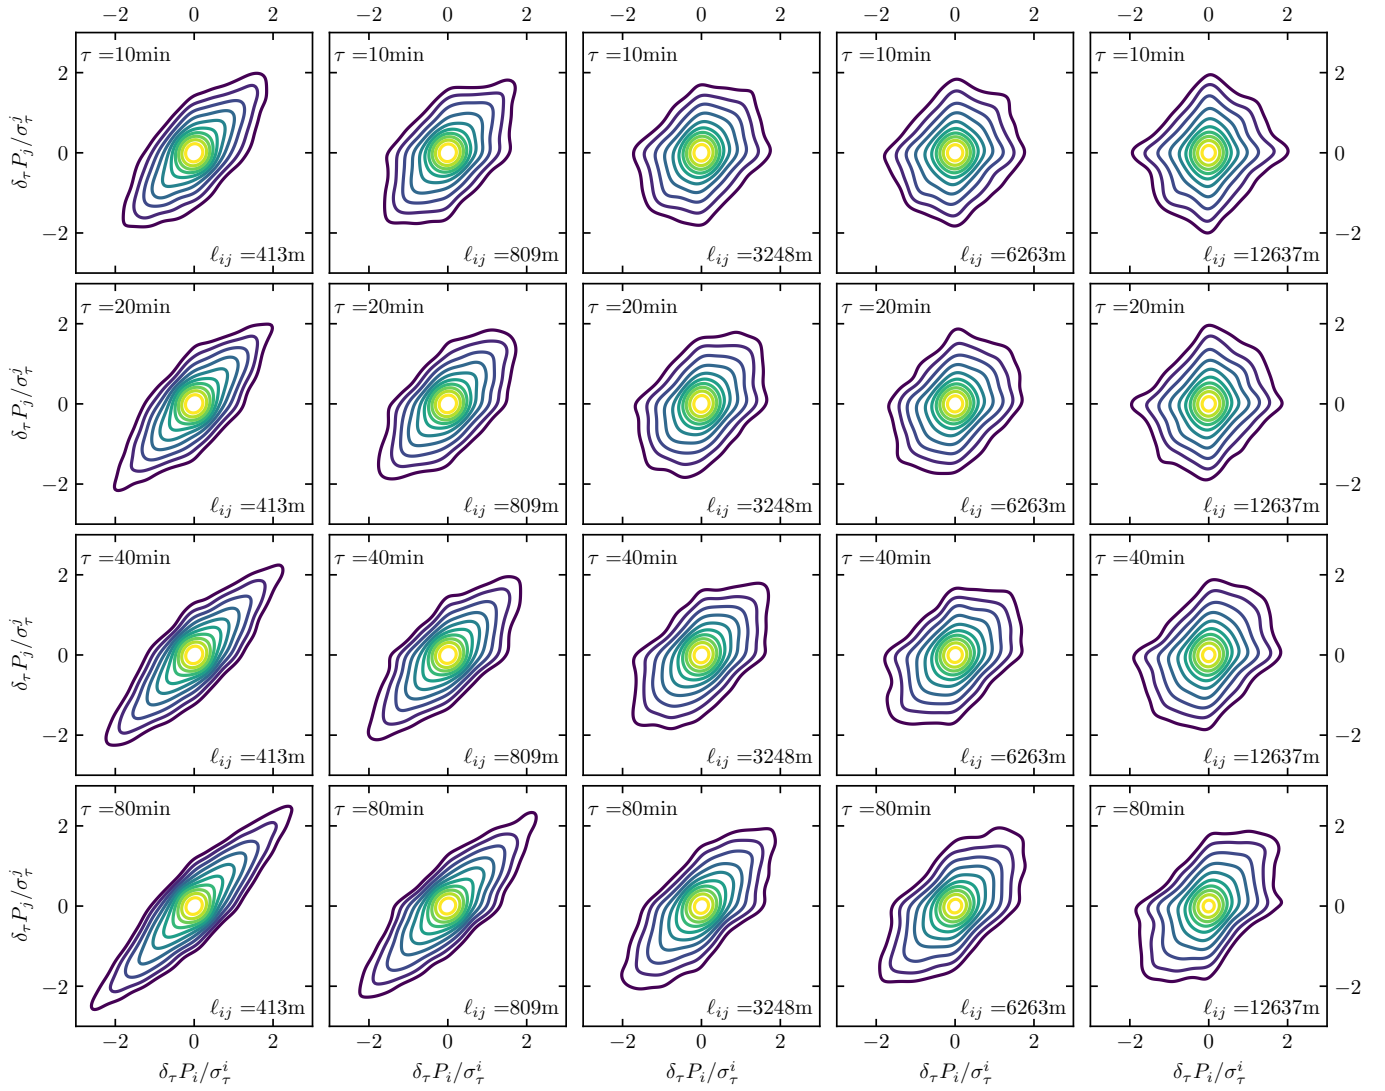

FIG. 7. Iso-density lines of power jumps bivariate distributions  $\rho(\delta_\tau P_i, \delta_\tau P_j)$ , with (top to down)  $\tau = 10\text{ min}, 20\text{ min}, 40\text{ min},$  and  $80\text{ min}$  and (left to right)  $\ell_{ij} = 413\text{m}, 809\text{m}, 3248\text{m}, 6263\text{m}, 12637\text{m}$

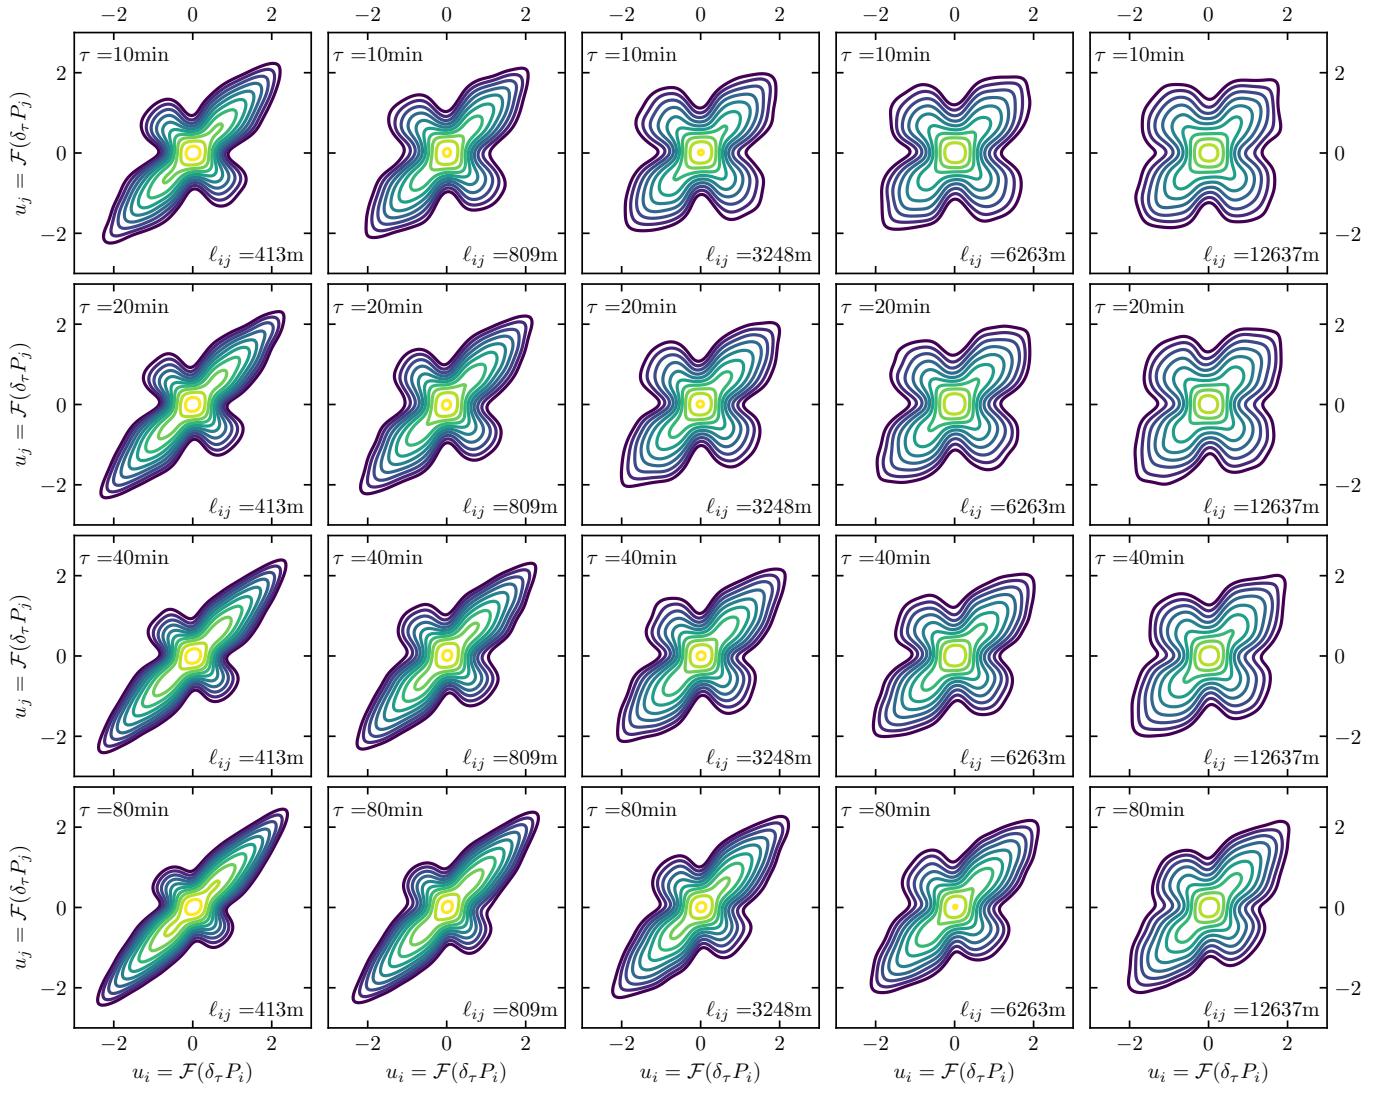

FIG. 8. Iso-density lines of Gaussianized power jumps bivariate distribution  $\rho(u_i, u_j) = \rho(\mathcal{F}(\delta_\tau P_i), \mathcal{F}(\delta_\tau P_j))$ , with (top to down)  $\tau = 10$  min, 20 min, 40 min, 80 min and (left to right)  $\ell_{ij} = 413$ m, 809m, 3248m, 6263m, 12637m
